# Supplementary material for: RobotFingerPrint: Unified Gripper Coordinate Space for Multi-Gripper Grasp Synthesis and Transfer
Source: arXiv:2409.14519 source file (2025-03-03)
Supplement: Supplementary file 1 [file appendix.tex]

\section*{APPENDIX}
\label{sec:appendix}

Supplementary Material  

Appendixes should appear before the acknowledgment.
